# Supplementary material for: On the anti-correlation between pericentric distance and inner dark matter density of Milky Way's dwarf spheroidal galaxies
Source: arXiv:2304.06611 source file (2023-04-13)
Supplement: Supplementary file 1 [file tables.tex]

\section{Tables}
